# Supplementary material for: Generalized and Scalable Optimal Sparse Decision Trees
Source: arXiv:2006.08690 source file (2022-11-22)
Supplement: Supplementary file 1 [file algorithm1.tex]

\definecolor{comment}{rgb}{0.2,0.4,0.2}
\def\comment#1{\textcolor{comment}{\textit{ // #1 }}}
\begin{algorithm}[]
\caption{GOSDT$(R, x, y, \lambda)$ \label{alg:gosdt_summary}}
\begin{small}
\begin{tabbing}
xxx \= xx \= xx \= xx \= xx \= xx \kill
0: \> \comment{Refer to Section \ref{Sec:notation} for definition of $R$ and $\lambda$} \\ 
1: \> \textbf{input:} $R$, $\x$, $\y$, $\lambda$ \comment{risk, samples, labels, regularizer} \\
2: \> \comment{Note all features have been binarized} \\
3: \> $s_{root} = [1,...,1]$ \comment{bitvector of all $n$ samples} \\
4: \> \comment{ Create a dictionary to store properties of problem $p$ } \\
5: \> $p_{root}.lower =$ Accuracy, where all samples of $s_{root}$ are classified correctly except minority-class equivalent points. 
%those with same feature values but different labels (the minority?) but without the complexity penalty of creating so many splits 
\\
6: \> $p_{root}.upper =$ Accuracy of applying the best single prediction to all points in $s_{root}$ with the complexity penalty of a single leaf. \\
7: \> $p_{root}.key = s_{root}$ \\

8: \> \textbf{if} $p_{root}$ fails Incremental Accuracy Bound, Leaf Accuracy Bound, and \textcolor{red}{or??} \textcolor{red}{ we don't have a support bound}Support Bound \textbf{then} \\
9: \> \> $p_{root}.lower = p_{root}.upper$ \\

10: \> $queue = [s_{root}]$ \comment{initialize queue with root} \\
11: \> $graph = \{s_{root}: p_{root}\}$ \comment{initialize dependency graph with root} \textcolor{red}{what is this notation?}\\

12: \> \textbf{while} $p_{root}.lower \neq p_{root}.upper$ \textbf{do} \\
13: \> \> \comment{pop key from queue and problem from graph} \\
14: \> \> $s \leftarrow queue.pop()$ \\
15: \> \> $p \leftarrow graph[s]$ \\
16: \> \> \textbf{if} $p.lower = p.upper$ \textbf{then} \\
17: \> \> \> \textbf{continue} \comment{problem solved} \\
18: \> \> \comment{Construction of child problems} \\ 
19: \> \> $(lower', upper') \leftarrow (\infty, \infty)$ \\
20: \> \> \textbf{for} $j \in \text{features} [1,..,M]$ \textbf{do}  \textcolor{red}{where does this for loop end?}\\ 21: \> \> \> \comment{create child nodes by adding a split on $j$}\\
22: \> \> \> $s_{\leftrm}=\{x_i:$ \text{feature $j$ of } $x_i$ is $0, x_i \in s\}$  \comment{data that goes left} \\
23: \> \> \> $s_{\rightrm}=\{x_i:$ \text{feature $j$ of } $x_i$ is $1, x_i \in s\}$ \comment{data that goes right}\\
24: \> \> \> \textbf{if} $s_{\leftrm} \notin graph$ \textbf{then}  \comment{we have not seen this problem yet, so must deal with it}\\
25: \> \> \> \> $p_{\leftrm} =$ Initialize $p_{\leftrm}$ with lower and upper for set $s_{\leftrm}$, similar to what we did for $p_{root}$ \\
26: \> \> \> \> \textbf{if} $p_{\leftrm}$ fails Incremental Accuracy Bound, Leaf Accuracy Bound, and Support Bound  \textcolor{red}{ check} \textbf{then} \\
27: \> \> \> \> \> $p_{\leftrm}.lower = p_{\leftrm}.upper$ \comment{we are done with this problem} \\
28: \> \> \> \> $p_{\leftrm}.key = s_{\leftrm}$ \\
29: \> \> \> \> $graph.insert(s_{\leftrm}, p_{\leftrm})$ \\
30: \> \> \> \textbf{if} $s_{\rightrm} \notin graph$ \textbf{then} \comment{handle right side similar to the way we handled left side} \\
31: \> \> \> \> $p_{\rightrm} =$ Initialize $p_{\rightrm}$ with lower and upper for set $s_{\rightrm}$, similar to what we did for $p_{root}$ \\
32: \> \> \> \> \textbf{if} $p_{\rightrm}$ fails Incremental Accuracy Bound, Leaf Accuracy Bound, and Support Bound \textcolor{red}{ check} \textbf{then} \\
33: \> \> \> \> \> $p_{\rightrm}.lower = p_{\rightrm}.upper$ \\
34: \> \> \> \> $p_{\rightrm}.key = s_{\rightrm}$ \\
35: \> \> \> \> $graph.insert(s_{\rightrm}, p_{\rightrm})$ \\

36: \> \> \> $p_{\leftrm} = graph[s_{\leftrm}]$\\
37: \> \> \> $p_{\rightrm} = graph[s_{\rightrm}]$\\

38: \> \> \> $lower' \leftarrow \min(lower', p_{\leftrm}.lower + p_{\rightrm}.lower)$ \comment{calculate bounds}\\
39: \> \> \> $upper' \leftarrow \min(upper', p_{\leftrm}.upper + p_{\rightrm}.upper)$ \\

40: \> \> \comment{Propagation: update upper and lower bounds} \\
41: \> \> \textbf{if} $p.lower \neq lower'$ \textbf{or} $p.upper \neq upper'$  \textbf{then} \textcolor{red}{is this in the for loop?}\\
42: \> \> \> $(p.lower, p.upper) \leftarrow (lower', upper')$ \\
43: \> \> \> \textbf{for} $p_{\rm parent}$ of $p$ \textbf{do} \comment{encourage update for the parent by making it high priority} \\
44: \> \> \> \> $queue.push(p_{\rm parent}.key, HIGH\_PRIORITY)$  \comment{$p_{\rm parent}.key$ is $s_{\rm parent}$}\\

45: \> \> \comment{Delegation} \textcolor{red}{what are you doing here? are you doing the for loop again? Why didn't you just store it when you found it? Some comments here would be useful}\\
46: \> \> \textbf{if} $p.lower < p.upper$ \textbf{then} \\ 
47: \> \> \> $(lower', upper') \leftarrow (\infty, \infty)$ \\
48: \> \> \textbf{for} $j \in \text{features} [1,..,M]$ \textbf{do} \\
49: \> \> \> $s_{\leftrm}\leftarrow\{x_i:$ \text{feature $j$ of } $x_i$ is $0, x_i \in s\}$\\
50: \> \> \> $s_{\rightrm}\leftarrow\{x_i:$ \text{feature $j$ of } $x_i$ is $1, x_i \in s\}$\\
51: \> \> \> $p_{\leftrm} \leftarrow graph[s_{\leftrm}]$\\
52: \> \> \> $p_{\rightrm} \leftarrow graph[s_{\rightrm}]$\\
53: \> \> \> \> $lower' \leftarrow \min(lower', p_{\leftrm}.lower + p_{\rightrm}.lower)$ \\
54: \> \> \> \> $upper' \leftarrow \min(upper', p_{\leftrm}.upper + n_{\rightrm}.upper)$ \\
55: \> \> \> \> \textbf{if} $lower' < upper'$ \textbf{and} $lower' \le p.upper$ \textbf{then} \\
56: \> \> \> \> \> $queue.push(s_{\leftrm}, LOW\_PRIORITY)$ \\
57: \> \> \> \> \> $queue.push(s_{\rightrm}, LOW\_PRIORITY)$ \\
58: \> \> \textbf{return} \\
\end{tabbing}
\end{small}
\end{algorithm}
