# Supplementary material for: Generalized and Scalable Optimal Sparse Decision Trees
Source: arXiv:2006.08690 source file (2022-11-22)
Supplement: Supplementary file 2 [file min_exploration.tex]

\begin{algorithm}
\caption{\textcolor{red!55!white}{MinExploration}$(G, Q, R, x, y, \lambda) \rightarrow$ None }
\begin{minipage}{1.0\linewidth}
\begin{tabbing}
xxx \= xxx \= xxx \= xxx \kill
\textbf{input:} $G, Q, R, x, y, \lambda$ \comment{dependency graph, evaluation queue, objective risk function, samples, labels, regularizer} \\
% \textbf{input:} $Q$ \comment{queue of problems to evaluate} \\
% \textbf{input:} $R$ \comment{objective risk function to optimize} \\
% \textbf{input:} $x$ \comment{observed training features} \\
% \textbf{input:} $y$ \comment{observed training labels} \\
% \textbf{input:} $\lambda$ \comment{regularization coefficient} \\

$key \leftarrow (x, y, -1)$ \comment{key for graph look-up} \\
$(l_0,u_0) \leftarrow V[key_{child}]$ \comment{bounds at current time-step} \\
$(V, E) \leftarrow G$ \\

% \comment{decompose problem into a set of subproblems} \\
% \comment{problems and subproblems form a parent-child relation} \\
\comment{breadth first search through dependency graph}\\
\textbf{if} $V[key].explored = False$ \textbf{then} \\
\> $V[key].explored \leftarrow True$\\
\> \comment{create a child subproblem for each feature index $j$} \\
\> \textbf{for} each feature $j \in [1, M]$ \textbf{do} \\
\> \> \comment{expand the graph to include the child} \\
\> \> \comment{initially inherit bounds of the parent problem} \\
\> \> $V[(x, y, j)] \leftarrow (l_0, u_0)$ \comment{initialize graph vertex} \\
\> \> $E[(x, y, -1), (x, y, j)] \leftarrow True$ \comment{initialize edge} \\
\> \textbf{endfor} \\
\textbf{endif} \\

\textbf{return}
\end{tabbing}
\end{minipage}
\end{algorithm}
