# Supplementary material for: Generalized and Scalable Optimal Sparse Decision Trees
Source: arXiv:2006.08690 source file (2022-11-22)
Supplement: Supplementary file 3 [file min_reduction.tex]

\begin{algorithm}
\caption{\textcolor{red!55!blue}{MinReduction}$(G, Q, R, x, y, \lambda) \rightarrow (l, u)$ }
\begin{minipage}{1.0\linewidth}
\begin{tabbing}
xxx \= xxx \= xxx \= xxx \kill
\textbf{input:} $G, Q, R, \x,\y, \lambda$ \comment{dependency graph, priority queue, risk, samples, labels, regularizer} \\
%\textbf{input:} $Q$ \comment{queue of problems to evaluate} \\
%\textbf{input:} $R$ \comment{objective risk function to optimize} \\
%\textbf{input:} $x$ \comment{observed training features} \\
%\textbf{input:} $y$ \comment{observed training labels} \\
%\textbf{input:} $\lambda$ \comment{regularization coefficient} \\
\textbf{output:} $l, u$ \comment{lower and upper bound based on children} \\
%\textbf{output:} $u$ \comment{upperbound based on children} \\
$key \leftarrow (x, y, -1)$ \comment{key for graph look-up} \\
$(l_0,u_0) \leftarrow V[key_{child}]$ \comment{bounds at current time-step} \\
$(V, E) \leftarrow G$ \\

\textcolor{red}{is this a typo? should it be l0, u0}\\
$(l, u) \leftarrow (u_0, u_0)$ \\
\comment{check for updates to bounding interval from children} \\
\textbf{for} $c \in G.children(key)$ \textbf{do} \\
\> $(l_c,u_c) \leftarrow V[c]$ \comment{child's bounds at current time-step} \\
\> \comment{update bounds if a more precise bound is found} \\
\> \textbf{if} $V[c].cancelled = False$ \textbf{then} \\
\> \> $l \leftarrow min(l, l_c)$ \\
\> \> $u \leftarrow min(u, u_c)$ \\
\> \textbf{endif} \\
\textbf{endfor} \\
\textbf{return} $(l, u)$
%\textbf{return}
\end{tabbing}
\end{minipage}
\end{algorithm}
