# Supplementary material for: Generalized and Scalable Optimal Sparse Decision Trees
Source: arXiv:2006.08690 source file (2022-11-22)
Supplement: Supplementary file 4 [file min_task.tex]

\begin{algorithm}
\caption{MinTask$(G, Q, R, x, y, \lambda) \rightarrow$ None \textcolor{red}{when you call this function?}}
\begin{minipage}{1.0\linewidth}
\begin{tabbing}
xxx \= xxx \= xxx \= xxx \kill
\textbf{input:} $G, Q, R, \x, \y, \lambda$ \comment{dependency graph, priority queue queue, risk, samples, labels, regularizer} \\
% \textbf{input:} $Q$ \comment{queue of problems to evaluate} \\
% \textbf{input:} $R$ \comment{objective risk function to optimize} \\
% \textbf{input:} $x$ \comment{observed training features} \\
% \textbf{input:} $y$ \comment{observed training labels} \\
% \textbf{input:} $\lambda$ \comment{regularization coefficient} \\

$key \leftarrow (x, y, -1)$ \comment{key for graph look-up} \\
$(l_0,u_0) \leftarrow V[key_{child}]$ \comment{bounds at current time-step} \\
$(V, E) \leftarrow G$ \\

\textcolor{red}{clarification--what's resolved/cancelled?}\\
\textbf{if} $V[key].resolved = True$ or $V[key].cancelled = True$ \textbf{then} \\ 
\> \textbf{return} \\
\textbf{endif}

\comment{expand graph with subproblems} \\
\textcolor{red!55!}{MinExploration}$(G, Q, R, \x, \y, \lambda)$\\

\comment{determine if problem can be pruned} \\

\textbf{if} \textcolor{red}{ AccuracyLowerBound$(R, x, y, \lambda) = False$ } \textbf{then} \\
\> $V[key].cancelled \leftarrow True$  \\
\textbf{else} \\
\> $V[key].cancelled \leftarrow False$ \\
\textbf{endif} \\

% $V[key].cancelled \leftarrow$ MinCancellation$(G, Q, R, x, y, \lambda)$ \\
\textbf{if} $V[key].cancelled = True$ \textbf{then} \\
\> \comment{notify parents of cancellation and terminate self} \\
\> $Q.EnqueueAll(G.parents(key))$ \\
\> \textbf{return} \\
\textbf{endif} \\

 \comment {update vertex with new bounds} \\
$V[key] \leftarrow$ \textcolor{red!55!blue}{MinReduction}$(G, Q, R, \x, \y, \lambda)$ \\

\comment{determine if children can be pruned} \\
$V[key].resolved \leftarrow$ \textcolor{blue!55!white}{MinResolution}$(G, Q, R, x, y, \lambda)$ \\
\textbf{if} $V[key].resolved = True$ or $l \ne l_0$ or $u \ne u_0$ \textbf{then} \\
\> \comment{notify parents of new bounds} \\
\> $Q.EnqueueAll(G.parents(key))$ \\
\> \textbf{if} $V[key].resolved = True$ \textbf{then} \\
\> \> \textbf{return} \\
\> \textbf{endif} \\
\textbf{endif} \\
\comment{enqueue children for further computation} \\

MinDelegate$(G, Q, R, x, y, \lambda)$ \\

\textbf{return}
\end{tabbing}
\end{minipage}
\end{algorithm}
