# Supplementary material for: Generalized and Scalable Optimal Sparse Decision Trees
Source: arXiv:2006.08690 source file (2022-11-22)
Supplement: Supplementary file 5 [file sum_exploration.tex]

\begin{algorithm}
\caption{SumExploration$(G, Q, R, x, y, j, \lambda) \rightarrow$ None }
\begin{minipage}{1.0\linewidth}
\begin{tabbing}
xxx \= xxx \= xxx \= xxx \kill
\textbf{input:} $G, Q,R,\x,\y,\lambda, j$ \comment{dependency graph, priority queue, samples, labels, regularizer, feature index} \\
% \textbf{input:} $G$ \comment{graph of problem state} \\
% \textbf{input:} $Q$ \comment{queue of problems to evaluate} \\
% \textbf{input:} $R$ \comment{objective risk function to optimize} \\
% \textbf{input:} $x$ \comment{observed training features} \\
% \textbf{input:} $y$ \comment{observed training labels} \\
% \textbf{input:} $j$ \comment{feature index used to partition $x$} \\
% \textbf{input:} $\lambda$ \comment{regularization coefficient} \\

$key \leftarrow (x, y, j)$ \comment{key for graph look-up} \\
$(l_0,u_0) \leftarrow V[key_{child}]$ \comment{bounds at current time-step} \\
$(V, E) \leftarrow G$ \\

\comment{breadth first search through dependency graph} \\
\textbf{if} $V[key].explored = False$ \textbf{then} \\
\> $V[key].explored \leftarrow True$\\
\> \textbf{for} $v \in \{0,1\}$ \textbf{do} \\
\> \> \comment{create a child subproblem for each feature index $j$} \\
\> \> \comment{select the subset of $x$ where column $j$ equals $v$} \\
\> \> $x_v \leftarrow x[x[:,j] = v]$ \\
\> \> $y_v \leftarrow y[x[:,j] = v]$ \\
\> \> $key_v \leftarrow (x_v, y_v)$ \\
\> \> \textbf{if} $key_v \not\in V$ \textbf{then} \\
\> \> \> \comment{initialize vertex} \\
\> \> \> $V[key_v] \leftarrow$ InitialBounds$(R, x_v, y_v, \lambda)$ \\
\> \> \textbf{endif} \\
\> \> $E[key, key_v] \leftarrow v$ \comment{initialize edge} \\
\> \textbf{endfor}
\textbf{endif} \\

\textbf{return} \\
\end{tabbing}
\end{minipage}
\end{algorithm}
