# Supplementary material for: Generalized and Scalable Optimal Sparse Decision Trees
Source: arXiv:2006.08690 source file (2022-11-22)
Supplement: Supplementary file 6 [file variable_selection.tex]

Although our algorithm is able to deal with the continuous features when building decision trees, we believe that if some features are proved to be unimportant, then it won't be used to build the optimal tree. 

We adapt the definition of \textit{Rashomon} set and \textit{model class reliance (MCR)} from \cite{fisher2018}. \textit{Rashomon} set is the set of prediction models that provide near optimal accuracy. Given a reference model $f_{\rm ref}$, we define a population $\epsilon$-Rashomon set denoted as $\mathcal{R}(\epsilon)$ as the subset of models
with expected loss no more than $\epsilon$ above that of $f_{\rm ref}$. Let $\Psi$ be a collection of variables of interests, and $\Tilde{X}$ be a collection of other covariates. Let $\ell$ be any nonnegative loss function. Given a model $f$, the permutation error is defined as 
\begin{equation}
    e_{\rm switch}(f) = \frac{1}{N(N-1)}\sum_{i=1}^N \sum_{j \neq i} \ell \{f, (y_{[j]}, \Tilde{X}_{[j,\cdot]}, \Psi_{[i,\cdot]})\}
\end{equation}
and standard error as
\begin{equation}
    e_{\rm orig}(f) = \frac{1}{N}\sum_{i=1}^N \ell \{f, (y_{[i]}, \Tilde{X}_{[i,\cdot]}, \Psi_{[i,\cdot]})\}.
\end{equation}
Then the model reliance (MR) is defined as 
\begin{equation}
   MR(f) = \frac{e_{\rm switch}(f)}{e_{\rm orig}(f)} 
\end{equation}
and the model class reliance is defined as 
\begin{equation}
    [MCR_{-(\epsilon)}, MCR_{+(\epsilon)}] = [\min_{f\in \mathcal{R}(\epsilon)}MR(f), \max_{f\in \mathcal{R}(\epsilon)}MR(f)]
\end{equation}

%First, we review a core measure of how much an individual prediction model relies on covariates of interest for its accuracy, which we call model reliance (MR).

%model class reliance (MCR) as the highest and lowest degree to which any well-performing model within a given class may rely on a variable of interest for prediction accuracy

\begin{theorem}\label{thm:vs}
Let $\mathcal{R}(\epsilon)$ be the Rashomon set, $\Psi$ be the collection of variables that are not heavily used in near optimal models, that is $MCR_{+(\epsilon)} < 1+2\lambda$, where $\lambda$ is the regularization term, and $\Tilde{X}$ be the collection of other variables. Let $\ell$ be the misclassification error. Let $d=(d_{\fix}, \delta_{\fix}, d_{\splitrm}, \delta_{\splitrm}, K, H_d)$ be a tree in the Rashomon set and do not use any variable in $\Psi$. Let $l_u \in d_{\splitrm}$ be a leaf that can be further split. Denote $n^+_u$ be the number of positive samples ($n^-_u$ be the number of negative samples) captured by $l_u$. Suppose $n^+_u \approx n^-_u$. Split $l_u$ by a variable $\psi$ s.t. $\psi \in \Psi$ and generate two leaves $l_v$ and $l_{v'}$. The new tree is also in the Rashomon set, but the incremental accuracy is smaller than $\lambda$, that is $e_{orig}({d})-e_{orig}({d'}) < \lambda$.
\end{theorem}

\begin{proof}
Let $n^+_u\ (n^-_u), n^+_v\ (n^-_v)$ and $n^+_{v'}\ (n^-_{v'})$ be the number of positive (negative) samples captured by $l_u$, $l_v$, and $l_{v'}$ respectively. Let $e_{\fix}$ be the error of all other leaves in tree $d$ except $l_u$, and let $N_{\psi}$ be the number of samples with $\psi = 0$. When $\hat{y}^{(\leaf)}_v=\hat{y}^{(\leaf)}_{v'}$, $e_{orig}({d})-e_{orig}({d'}) = 0 \leqslant \lambda$. When $\hat{y}^{(\leaf)}_v \neq \hat{y}^{(\leaf)}_{v'}$, there are four different situations. We only show one here and others can be proved in the same way. When $\hat{y}^{(\leaf)}_u = 1, \hat{y}^{(\leaf)}_v=0, \hat{y}^{(\leaf)}_{v'}=1$, since tree $d$ doesn't use any variable in $\Psi$,
\begin{equation}
    e_{\rm orig}(d) = e_{\rm switch}(d) = e_{\fix}+\frac{n^-_u}{N} = e_{\fix}+e_{u}
\end{equation} 
where $e_u$ is the error of leaf $l_u$. 
For tree $d'$, 
$$e_{\rm orig}(d')=e_{fix}+e_{v}+e_{v'}$$ where $e_v$ is the error of leaf $l_v$ and $e_{v'}$ is the error of leaf $l_{v'}$. 
$$e_{\rm switch}(d') = e_{\fix} + \frac{1}{N(N-1)}(N_{\psi}n^+_u - n^+_v + (N-N_\psi)n^-_u - n^-_{v'}) =: e_{\fix} + e_{\rm perm}$$
$$e_{\rm switch}(d')-e_{\rm orig}(d)=e_{\rm perm}-e_u = \frac{N_{\psi}-1}{N-1}\frac{n^+_u-n^-_u}{N}+\frac{n^+_{v'}-n^-_{v'}}{N(N-1)}$$
Since $n^+_u\approx n^-_u$ and $\frac{n^+_{v'}-n^-_{v'}}{N(N-1)}$ is very small, $e_{perm} \approx e_u$ and $e_{switch}(d')\approx e_{orig}(d)$. We can get the same results in other three situations. Meanwhile, since $MCR_{+(\epsilon)} < 1+2\lambda$, then 
\begin{eqnarray*}
&&\frac{e_{\rm switch}(d')}{e_{\rm orig}(d')} < 1+2\lambda\\ &\Rightarrow& \frac{e_{\fix}+e_{\rm perm}}{e_{\fix}+e_v+e_{v'}} < 1+2\lambda\\
&\Rightarrow& 1+\frac{e_{\rm perm}-e_v-e_{v'}}{e_{\fix}+e_v+e_{v'}} < 1+2\lambda\\
&\Rightarrow& e_u - e_v-e_{v'} < 2\lambda(e_{\fix}+e_v+e_{v'}) \leqslant 2\lambda \times 0.5 = \lambda\\
&\Rightarrow& e_{\rm orig}({d})-e_{\rm orig}({d'}) < \lambda
\end{eqnarray*}
\end{proof}

\begin{theorem}\label{thm:vs_acc}
Adopt all notations, definitions, and assumptions in Theorem \ref{thm:vs}. Let $a_u$, $a_{v}$, $a_{v'}$ be the fraction of correctly classified data in $l_u$, $l_v$, $l_{v'}$ respectively, i.e., 
\begin{equation}
    a_u = \frac{1}{N}\sum_{i=1}^N {\rm cap}(x_i, l_u) \wedge \mathbf{1}[\hat{y}^{(\leaf)}_u = y_i]
\end{equation}
Suppose $|a_v-a_{v'}| \geq a_u-\lambda$, then the feature $\psi$ won't be used to split the leaf.
\end{theorem}

\begin{proof}
According to Theorem \ref{thm:vs}, $a_v+a_{v'} - a_u < \lambda$. Suppose $a_v \geqslant a_{v'}$, $\lambda > a_v+a_{v'}-a_u \geq 2a_{v'}-\lambda$, then we can get $a_{v'} < \lambda$. 
\end{proof}

According to the lower bound on classification accuracy in OSDT \citep{HuRuSe2019}, if a feature does not have the minimum fraction of correctly classified data for points that go to that leaf, then we can exclude that feature further down the tree extending that leaf. The feature will be excluded anywhere below the leaf. Therefore, if a feature is proved to be unimportant by other near optimal models, for some datasets we can exclude this feature in constructing the optimal decision trees.
