# Supplementary material for: Generalized and Scalable Optimal Sparse Decision Trees
Source: arXiv:2006.08690 source file (2022-11-22)
Supplement: Supplementary file 7 [file configuration.tex]

\definecolor{comment}{rgb}{0.2,0.4,0.2}
