# Supplementary material for: Generalized and Scalable Optimal Sparse Decision Trees
Source: arXiv:2006.08690 source file (2022-11-22)
Supplement: Supplementary file 8 [file initial_bounds.tex]

\begin{algorithm}
\caption{\textcolor{purple}{InitialBounds}$(R, x, y, \lambda) \rightarrow (l, u)$ }
\begin{minipage}{1.0\linewidth}
\begin{tabbing}
xxx \= xxx \= xxx \kill
\textbf{input:} $R,\x,\y,\lambda$ \comment{risk, samples, labels, regularizer} \\
\textbf{output:} $l, u$ \comment{lower bound and upper bound of $min(x, y, \lambda)$} \\
\comment{sample the solution space using an optimal stump} \\
$(d, r) \leftarrow$ \textcolor{cyan}{OptimalStump}$(R, \x, \y, \lambda)$ \\
\textcolor{red}{// room for improvement using smarter sampling methods?} \\
\comment{sample upperbounds the objective in the solution space} \\
$u \leftarrow r$ \\
\comment{compute lowerbound using equivalent points bound} \\
$l \leftarrow$ \textcolor{red}{EquivalentPointLowerbound$(R, x, y, \lambda)$} \\
\textbf{return} $(l, u)$
\end{tabbing}
\end{minipage}
\end{algorithm}
