# Supplementary material for: Generalized and Scalable Optimal Sparse Decision Trees
Source: arXiv:2006.08690 source file (2022-11-22)
Supplement: Supplementary file 9 [file min_cancellation.tex]

\begin{algorithm}
\caption{MinCancellation$(G, Q, R, x, y, \lambda) \rightarrow c$ }
\begin{minipage}{1.0\linewidth}
\begin{tabbing}
xxx \= xxx \= xxx \= xxx \kill
\textbf{input:} $G$ \comment{graph of problem state} \\
\textbf{input:} $Q$ \comment{queue of problems to evaluate} \\
\textbf{input:} $R$ \comment{objective risk function to optimize} \\
\textbf{input:} $x$ \comment{observed training features} \\
\textbf{input:} $y$ \comment{observed training labels} \\
\textbf{input:} $\lambda$ \comment{regularization coefficient} \\
\textbf{output:} $c$ \comment{boolean indicating this problem is pruned} \\
$key \leftarrow (x, y, -1)$ \comment{key for graph look-up} \\
\comment{determine if problem can be pruned} \\
\textbf{if} \textcolor{red}{ AccuracyLowerBound$(R, x, y, \lambda) = False$ } \textbf{then} \\
\> \textbf{return} $True$ \\
\textbf{endif} \\
\textbf{return} $False$\\
\end{tabbing}
\end{minipage}
\end{algorithm}
