# Supplementary material for: Generalized and Scalable Optimal Sparse Decision Trees
Source: arXiv:2006.08690 source file (2022-11-22)
Supplement: Supplementary file 10 [file min_delegation.tex]

\begin{algorithm}
\caption{MinDelegation$(G, Q, R, x, y, \lambda) \rightarrow$ None }
\begin{minipage}{1.0\linewidth}
\begin{tabbing}
xxx \= xxx \= xxx \= xxx \= xxx \kill
\textbf{input:} $G, Q, R, x, y, \lambda$ \comment{dependency graph, evaluation queue, objective risk function, samples, labels, regularizer} \\
% \textbf{input:} $Q$ \comment{queue of problems to evaluate} \\
% \textbf{input:} $R$ \comment{objective risk function to optimize} \\
% \textbf{input:} $x$ \comment{observed training features} \\
% \textbf{input:} $y$ \comment{observed training labels} \\
% \textbf{input:} $\lambda$ \comment{regularization coefficient} \\

$key \leftarrow (x, y, -1)$ \comment{key for graph look-up} \\
$(l,u) \leftarrow V[key_{child}]$ \comment{bounds at current time-step} \\
$(V, E) \leftarrow G$ \\
\comment{enqueue children to delegate work} \\
\textbf{if} $V[key].delegated = False$ \textbf{then} \\
\> $V[key].delegated \leftarrow True$ \\
\> \textbf{for} $c \in G.children(key)$ \textbf{do} \\
\> \comment{only delegate children if they are not resolved} \\
\> \comment{only delegate children whose bounds overlap with the current bound} \\
% \> \comment{contribute to the current bound} \\
\> \> \textbf{if} $V[c].resolved = False$ \textbf{then} \\
\> \> \> $(l_c, u_c) \leftarrow V[c]$ \\
\> \> \>\textbf{if} $l_c \le u$ \textbf{then} \\
\> \> \> \>  $Q.push(c)$ \\
\> \> \> \textbf{endif} \\
\> \> \textbf{endif} \\
\> \textbf{endfor} \\

\textbf{return}
\end{tabbing}
\end{minipage}
\end{algorithm}
