# Supplementary material for: Generalized and Scalable Optimal Sparse Decision Trees
Source: arXiv:2006.08690 source file (2022-11-22)
Supplement: Supplementary file 12 [file optimal_stump.tex]

\begin{algorithm}
\caption{\textcolor{cyan}{OptimalStump}$(R, x, y, \lambda) \rightarrow (d, r)$ }
\begin{minipage}{1.0\linewidth}
\begin{tabbing}
xxx \= xxx \= xxx \kill
\textbf{input:} $R, \x, \y, \lambda, d, r$ \comment{risk, samples, labels, regularizer, optimal decision stump, objective risk value of $d$} \\
% \textbf{input:} $d, r$ \comment{optimal decision stump, objective risk value of $d$}
% \textbf{input:} $x$ \comment{observed training features} \\
% \textbf{input:} $y$ \comment{observed training labels} \\
% \textbf{input:} $\lambda$ \comment{regularization coefficient} \\
% \textbf{output:} $d$ \comment{optimal decision stump} \\
% \textbf{output:} $r$ \comment{objective risk value of $d$} \\

\comment{compute the frequency of positive and negative labels} \\
$n \leftarrow \sum_{i=1}^{N}\mathbbm{1}[y_i = 0]$ \\
$p \leftarrow \sum_{i=1}^{N}\mathbbm{1}[y_i = 1]$ \\

\comment{build decision stump favoring the most frequent label} \\
$d \leftarrow (-1, \mathbbm{1}\{n \ge p\})$ \textcolor{red}{what is the -1 here for? Where is the more frequent label mentioned?}\\
\textbf{return} $(d, R(d, \x, \y, \lambda))$
\end{tabbing}
\end{minipage}
\end{algorithm}
