# Supplementary material for: Generalized and Scalable Optimal Sparse Decision Trees
Source: arXiv:2006.08690 source file (2022-11-22)
Supplement: Supplementary file 13 [file optimize.tex]

\begin{algorithm}
\caption{Optimize$(R, x, y, \lambda$) $\rightarrow$ $D$ \textcolor{red}{When do you call this?}} 
\begin{minipage}{1.0\linewidth}
\begin{tabbing}
xxx \= xxx \= xxx \kill
\textbf{input:} $R, \x, \y, \lambda$ \comment{risk, samples, labels, regularizer} \\
\textbf{output:} $D$ \comment{Set of optimal decision trees} \\

$key \leftarrow (x, y, -1)$ \comment{Key to main problem} \\
$(l, u) \leftarrow$ \textcolor{purple}{InitialBounds}$(R, x, y, \lambda)$ \comment{Compute bounds} \\

\comment{Create dependency graph to memoize results} \\
$V \leftarrow \{\}$ \comment{Vertices correspond to problems} \\
$V[key] \leftarrow (l, u)$ \comment{store bounds} \\
$E \leftarrow \{\}$ \comment{Edges correspond to dependencies} \\
$G \leftarrow (V, E)$ \comment{Store vertices and edges in graph} \\
\comment{Create queue to schedule problems as tasks} \\
$Q \leftarrow \{ key \}$ \comment{Enqueue main problem} \\

\textbf{while} $V[key_{0}].resolved = False$ \textbf{do} \comment{While we haven't fully solved the base problem} \\
\> $key_t \leftarrow Q.Dequeue()$ \comment{Dequeue the next problem} \\
\> $(x_t, y_t, j_t) \leftarrow key_t$ \\
\> \textbf{if} $j_t = -1$ \textbf{do} \comment{Evaluate minimization} \\
\> \> MinTask$(G, Q, R, x_t, y_t, \lambda)$ \\
\> \textbf{else} \comment{Evaluate summation} \\
\> \> SumTask$(G, Q, R, x_t, y_t, j_t, \lambda)$ \\
\> \textbf{endif} \\
\textbf{endwhile} \\
\textbf{return} Model(G, root)
\end{tabbing}
\end{minipage}
\end{algorithm}
