# Supplementary material for: Generalized and Scalable Optimal Sparse Decision Trees
Source: arXiv:2006.08690 source file (2022-11-22)
Supplement: Supplementary file 16 [file sum_reduction.tex]

\begin{algorithm}
\caption{SumReduction$(G, Q, R, x, y, \lambda, j) \rightarrow (l, u)$ }
\begin{minipage}{1.0\linewidth}
\begin{tabbing}
xxx \= xxx \= xxx \= xxx \kill
\textbf{input:} $G, Q,R,\x,\y,\lambda, j$ \comment{dependency graph, priority queue, samples, labels, regularizer, feature index} \\
%\textbf{input:} $G$ \comment{graph of problem state} \\
%\textbf{input:} $Q$ \comment{queue of problems to evaluate} \\
%\textbf{input:} $R$ \comment{objective risk function to optimize} \\
%\textbf{input:} $x$ \comment{observed training features} \\
%\textbf{input:} $y$ \comment{observed training labels} \\
%\textbf{input:} $j$ \comment{feature index used to partition $x$} \\
%\textbf{input:} $\lambda$ \comment{regularization coefficient} \\
\textbf{output:} $l, u$ \comment{lower and upper bound based on children} \\
%\textbf{output:} $u$ \comment{upperbound based on children} \\
$key \leftarrow (x, y, j)$ \comment{key for graph look-up} \\
$(l_0,u_0) \leftarrow V[key_{child}]$ \comment{bounds at current time-step} \\
$(V, E) \leftarrow G$ \\

$(l, u) \leftarrow (u_0, u_0)$ \\
\comment{check for updates to bounding interval from children} \\
\textbf{for} $c \in G.children(key)$ \textbf{do} \\
\> $(l_c,u_c) \leftarrow V[c]$ \comment{child's bounds at current time-step} \\
\> \comment{update bounds if a more precise bound is found} \\
\> $l \leftarrow l + l_c$ \\
\> $u \leftarrow u + u_c$ \\
\textbf{endfor} \\
\textbf{return} $(l, u)$

\textbf{return}
\end{tabbing}
\end{minipage}
\end{algorithm}
