# Supplementary material for: Generalized and Scalable Optimal Sparse Decision Trees
Source: arXiv:2006.08690 source file (2022-11-22)
Supplement: Supplementary file 17 [file sum_resolution.tex]

\begin{algorithm}
\caption{SumResolution$(G, Q, R, x, y, \lambda,j ) \rightarrow c$ }
\begin{minipage}{1.0\linewidth}
\begin{tabbing}
xxx \= xxx \= xxx \= xxx \kill
\textbf{input:} $G, Q,R,\x,\y,\lambda, j$ \comment{dependency graph, priority queue, samples, labels, regularizer, feature index} \\
%\textbf{input:} $Q$ \comment{queue of problems to evaluate} \\
%\textbf{input:} $R$ \comment{objective risk function to optimize} \\
%\textbf{input:} $x$ \comment{observed training features} \\
%\textbf{input:} $y$ \comment{observed training labels} \\
%\textbf{input:} $j$ \comment{feature index used to partition $x$} \\
%\textbf{input:} $\lambda$ \comment{regularization coefficient} \\
\textbf{output:} $c$ \comment{boolean indicating this problem is resolved} \\

$key \leftarrow (x, y, j)$ \comment{key for graph look-up} \\
$(l,u) \leftarrow V[key_{child}]$ \comment{bounds at current time-step} \\
$(V, E) \leftarrow G$ \\

\comment{determine if children can be pruned} \\
\textbf{if} \textcolor{red}{IncrementalAccuracyLowerBound$(l, u) = False$} \textbf{then} \\
\> \textbf{return} $True$ \\
\textbf{else if} \textcolor{red}{SupportLowerBound$(x) = False$} \textbf{then} \\
\> \textbf{return} $True$ \\
\textbf{else if} $l = u$ \textbf{then} \\
\> \textbf{return} $True$ \\
\textbf{endif} \\

\textbf{return} False
\end{tabbing}
\end{minipage}
\end{algorithm}
