# Supplementary material for: Generalized and Scalable Optimal Sparse Decision Trees
Source: arXiv:2006.08690 source file (2022-11-22)
Supplement: Supplementary file 18 [file sum_task.tex]

\begin{algorithm}
\caption{SumTask$(G, Q, R, x, y, j, \lambda) \rightarrow$ None }
\begin{minipage}{1.0\linewidth}
\begin{tabbing}
xxx \= xxx \= xxx \= xxx \kill
\textbf{input:} $G, Q,R,\x,\y,\lambda, j$ \comment{dependency graph, priority queue, samples, labels, regularizer, feature index} \\
% \textbf{input:} $Q$ \comment{queue of problems to evaluate} \\
% \textbf{input:} $R$ \comment{objective risk function to optimize} \\
% \textbf{input:} $x$ \comment{observed training features} \\
% \textbf{input:} $y$ \comment{observed training labels} \\
% \textbf{input:} $j$ \comment{feature index used to partition $x$} \\
% \textbf{input:} $\lambda$ \comment{regularization coefficient} \\

$key \leftarrow (x, y, j)$ \comment{key for graph look-up} \\
$(l_0,u_0) \leftarrow V[key_{child}]$ \comment{bounds at current time-step} \\
$(V, E) \leftarrow G$ \\

\textbf{if} $V[key].resolved = True$ or $V[key].cancelled = True$ \textbf{then} \\
\> \textbf{return} \\
\textbf{endif}

\comment{expand graph with subproblems} \\
SumExploration$(G, Q, R, x, y, j, \lambda)$\\

\comment{determine if problem can be pruned} \\
$V[key].cancelled \leftarrow$ SumCancellation$(G, Q, R, x, y, j, \lambda)$ \\
\textbf{if} $V[key].cancelled = True$ \textbf{then} \\
\> \comment{notify parents of cancellation and terminate self} \\
\> $Q.EnqueueAll(G.parents(key))$ \\
\> \textbf{return} \\
\textbf{endif} \\

\comment {update vertex with new bounds} \\
$V[key] =$ SumReduction$(G, Q, R, x, y, j, \lambda)$ \\

\comment{determine if children can be pruned} \\
$V[key].resolved \leftarrow$ SumResolution$(G, Q, R, x, y, j, \lambda)$ \\
\textbf{if} $V[key].resolved = True$ or $l \ne l_0$ or $u \ne u_0$ \textbf{then} \\
\> \comment{notify parents of new bounds} \\
\> $Q.EnqueueAll(G.parents(key))$ \\
\> \textbf{if} $V[key].resolved = True$ \textbf{then} \\
\> \> \textbf{return} \\
\> \textbf{endif} \\
\textbf{endif} \\
\comment{enqueue children for further computation} \\

SumDelegation$(G, Q, R, x, y, j, \lambda)$ \\

\textbf{return}
\end{tabbing}
\end{minipage}
\end{algorithm}

%\begin{algorithmic}
%\end{algorithmic}
