# Supplementary material for: Generalized and Scalable Optimal Sparse Decision Trees
Source: arXiv:2006.08690 source file (2022-11-22)
Supplement: Supplementary file 19 [file OldTextAboutIncrementalSimilarSupport.tex]

%For any two optimal trees $d$ and $D$ of the same support set $S$, same fixed leaves %$d_{\fix}$  and same split leaves %$d_{\split}$ but different splits at their roots:
%Let $\omega$ be defined as the normalized support of the samples that would move either from the left subtree to the right subtree or from the right subtree to the left subtree if $d$ were to be replaced with $D$. 
%Let $\epsilon_{--}$ be defined as the \textcolor{red}{uncertainty} over the set of points that are in the left subtree of both $d$ and $D$.
%Let $\epsilon_{++}$ be defined as the uncertainty over the set of points that are in the right subtree of both $d$ and $D$.
%The difference between the objectives $|R_{d} - R_{D}|$ at any time in the algorithm is bounded as follows:
%\begin{equation}
%|R_{d} - R_{D}| \le \omega + \epsilon_{++} + %\epsilon_{--}.
%\end{equation}


%\begin{proof}
%Let there be two optimal trees $d$ and $D$ each splitting the data set along slightly different boundaries, branching into into subtree pairs $(d_l, d_r)$ and $(D_l, D_r)$ respectively ($l$ and $r$ stand for ``left'' and ``right.'' The only difference between these trees is the split at the top of the tree. Denote $I(d_l)$ as the set of indices of observations \textcolor{red}{captured} by subtree $d_l$, with similar definitions for $I(d_r)$, $I(D_l)$, and $I(D_r)$. The algorithm computes a lower bound $R_d$ on the optimal risk of the trees as follows:
%\begin{equation} R_d 
%= \min_{\tilde{d}} R(\tilde{d}, \{x_i\}_i, \{y\}_i) 
%:= R_{d_l} + R_{d_r} \textrm{ where}\end{equation}
%\begin{equation} R_{d_l} := \min_{d'} R(d', x_{I(d_l)}, y_{I(d_+)}) \end{equation}
%\begin{equation} R_{d_r} := \min_{d'} R(d', x_{I(d_r)}, y_{I(d_r)}), \end{equation}
%where these minimization problems minimize the risk over all possible subtrees $d'$ using the data captured by the subtree's root, which is either $d_+$ or $d_-$ in the equations above. Similarly, for $D_+$ and $D_-$,
%\begin{equation} R_D = \min_{d'} R(d', x, y) = R_{D_+} + R_{D_-} \textrm{ where} \end{equation}
%\begin{equation} R_{D_+} = \min_{d'} R(d', x_{I(D_+)}, y_{I(D_+)}) \end{equation}
%\begin{equation} R_{D_-} = \min_{d'} R(d', x_{I(D_-)}, y_{I(D_-)}). \end{equation}




%$(x_{d_+}, y_{d_+})$ and $(x_{d_-}, y_{d_-})$ are the resulting subsets of $\{(x_i, y_i)\}_i$ when splitting based on the root of decision tree $d$, and $(x_{D_+}, y_{D_+})$ and $(x_{D_-}, y_{D_-})$ are the resulting subsets of $(x, y)$ when splitting based on the root of decision tree $D$.

We express the absolute difference between $R_{d}$ and $R_{D}$ as
\begin{equation} |R_{d} - R_{D}| = |R_{d_+} + R_{d_-} - R_{D_+} - R_{D_-}| \end{equation}
\begin{equation} |R_{d} - R_{D}| = |(R_{d_+} - R_{D_+}) + (R_{d_-} - R_{D_-})|\leq |R_{d_+} - R_{D_+}| + |R_{d_-} - R_{D_-}|. \end{equation}
We define four subsets of data, $I_{++}$, $I_{--}$, $I_{+-}$, and $I_{-+}$, as follows:
\begin{eqnarray*} 
I_{++} &=& \{i:  i\in I(d_+) \bigcap I(D_+)\}\\
I_{--} &=& \{i:  i\in I(d_+) \bigcap I(D_-)\}\\
I_{+-} &=& \{i:  i\in I(d_+) \bigcap I(D_-)\}\\
I_{-+} &=& \{i:  i\in I(d_-) \bigcap I(D_+)\}.
%(x_{d_+} \bigcap x_{D_+}, y_{d_+} \bigcap y_{D_+}) 
\end{eqnarray*}
%$(x_{++}, y_{++})$, $(x_{--}, y_{--})$, $(x_{+-}, y_{+-})$, $(x_{-+}, y_{-+})$ as follows
%\begin{equation*} (x_{++}, y_{++}) = (x_{d_+} \bigcap x_{D_+}, y_{d_+} \bigcap y_{D_+}) \end{equation*}
%\begin{equation*} (x_{--}, y_{--}) = (x_{d_-} \bigcap x_{D_-}, y_{d_-} \bigcap y_{D_-}) \end{equation*}
%\begin{equation*} (x_{+-}, y_{+-}) = (x_{d_+} \bigcap x_{D_-}, y_{d_+} \bigcap y_{D_-}) \end{equation*}
%\begin{equation*} (x_{-+}, y_{-+}) = (x_{d_-} \bigcap x_{D_+}, y_{d_-} \bigcap y_{D_+}). \end{equation*}
We define lower and upper bounds on objectives for $I_{++}$ and $I_{--}$, denoted $R_{++}^{\min}$, $R_{++}^{\max}$, $R_{--}^{\min}$, and $R_{++}^{\max}$, %$R_{+-}$, $R_{-+}$ over each of the four sets using bounding intervals and define uncertainty values over the interval
\begin{eqnarray*} 
R_{d_{++}}^{\min} &\leq \min_{d'} R(d', x_{I_{++}}, y_{I_{++}})\leq &R_{d_{++}}^{\max}\\
R_{d_{--}}^{\min} &\leq \min_{d'} R(d', x_{I_{--}}, y_{I_{--}})\leq &R_{d_{--}}^{\max},
\end{eqnarray*}
Denoting $\omega_{+-} = |I_{+-}|/N$ as the fraction of observations that are in the right subtree of $d$ and the left subtree of $D$, and denote $\omega_{-+}= |I_{-+}|/N$ as the fraction of observations in the left of $d$ and the right of $D$, thus $\omega=\omega_{+-}+\omega_{-+}$. 
We can use these new values to form bounds over $R_{d_+}$, $R_{d_-}$, $R_{D_+}$, and $R_{D_-}$:
\begin{eqnarray*} 
R_{++}^{\min} &\le R_{d_+} \le&  R_{++}^{\max} + \omega_{+-}, \\
R_{--}^{\min} &\le R_{d_-} \le&  R_{--}^{\max} + \omega_{-+}\\
R_{++}^{\min} &\le R_{D_+} \le&  R_{++}^{\max} + \omega_{+-}, \\
R_{--}^{\min} &\le R_{D_-} \le&  R_{--}^{\max} + \omega_{-+},
\end{eqnarray*}
where the upper bounds come from the possibility that all $I_{+-}$ points are misclassified or that all $I_{-+}$ points are misclassified. The lower bounds come from the possibility that all these points are classified correctly.
Combining, we have: 
\begin{eqnarray*}
|R_{d} - R_{D}| &\leq& |R_{d_+} - R_{D_+}| + |R_{d_-} - R_{D_-}| \\
&\leq& 
R^{\max}_{++} + \omega_{+-} - R^{\min}_{++} + R^{\max}_{--} + \omega_{-+} - R^{\min}_{--}\\
&=& R^{\max}_{++} - R^{\min}_{++} + R^{\max}_{--} - R^{\min}_{--} + \omega.
\end{eqnarray*}
This is the statement of the theorem.




%\begin{equation*} R_{++} \in [R_{++}^{\min}, R_{++}^{\max}] \end{equation*}
%\begin{equation*} R_{--} \in [R_{--}^{\min}, R_{--}^{\max}] \end{equation*}
%\begin{equation} R_{+-} \in [R_{+-}^{\min}, R_{+-}^{\max}] \end{equation}
%\begin{equation} R_{-+} \in [R_{-+}^{\min}, R_{-+}^{\max}] \end{equation}

%\begin{equation} \epsilon_{++} = R^{\max}_{++} - R^{\min}_{++} \end{equation}
%\begin{equation} \epsilon_{--} = R^{\max}_{--} - R^{\min}_{--} \end{equation}
%\begin{equation} \epsilon_{+-} = R^{\max}_{+-} - R^{\min}_{+-} \end{equation}
%\begin{equation} \epsilon_{-+} = R^{\max}_{-+} - R^{\min}_{-+}. \end{equation}
%We can use these new values to form bounds over $R_{d_+}$, $R_{d_-}$, $R_{D_+}$, $R_{D_-}$.
%\begin{equation} R_{++}^{\min} + R_{+-}^{\min} \le R_{d_+} \le  R_{++}^{\max} + R_{+-}^{\max} \end{equation}
%\begin{equation} R_{--}^{\min} + R_{-+}^{\min} \le R_{d_-} \le R_{--}^{\max} + R_{-+}^{\max} \end{equation}
%\begin{equation} R_{++}^{\min} + R_{-+}^{\min} \le R_{D_+} \le  R_{++}^{\max} + R_{-+}^{\max} \end{equation}
%\begin{equation} R_{--}^{\min} + R_{-+}^{\min} \le R_{D_-} \le  R_{--}^{\max} + R_{-+}^{\max} \end{equation}
%By combining these bounds with equation (46) we get the following bound
%\begin{equation} |R_{d} - R_{D}| \le \epsilon_{+-} + \epsilon_{-+} + \epsilon_{++} + \epsilon_{--} \end{equation}

%Define $(x_\omega, y_\omega)$ as the union of $(x_{+-},y_{+-})$ and $(x_{-+},y_{-+})$, which form the set of data that transferred from $d_+$ to $D_-$ or from $d_-$ to $D_+$ as a result of the difference in split across $d$ and $D$.
%\begin{equation} (x_\omega, y_\omega) = (x_{+-},y_{+-}) \cup (x_{-+},y_{-+}) \end{equation}
%Define $\omega$ as the number of samples in $(x_\omega, y_\omega)$
%\begin{equation} \omega = \| (x_\omega, y_\omega) \| = \| (x_{+-},y_{+-}) \| + \| (x_{-+},y_{-+}) \| \end{equation}
%Using the following inequalities
%\begin{equation} R_{+-}^{\max} \le \| (x_{+-},y_{+-}) \| \end{equation}
%\begin{equation} R_{-+}^{\max} \le \| (x_{-+},y_{-+}) \| \end{equation}
%We show that 
%\begin{equation} R_{+-}^{\max} + R_{-+}^{\max} \le \omega \end{equation}
%\begin{equation} |R_{d} - R_{D}| \le \omega + \epsilon_{++} + \epsilon_{--} \end{equation}
